# Supplementary material for: Risk of Transfer Learning and its Applications in Finance
Source: arXiv:2311.03283 source file (2023-11-06)
Supplement: Supplementary file 1 [file appendix.tex]

\newpage

\begin{center}
{\Large \bf {\centering Appendix}}
\end{center}

\appendix

\section{Mathematical Proofs}

\subsection{Proof of Theorem \ref{thm:existence}}\label{app:thm-exist}
We will show that the optimization problem \eqref{eq: doub-trans} is well-defined in the sense that an optimal pair of transport mappings $(T^{X,*},T^{Y,*})$ for \eqref{eq: doub-trans} is obtainable, under certain regularity conditions. More specifically, we will focus on the following type of loss function $\LL_T$. 

\begin{defn}[Proper loss function]
   Let $(X,Y)$ be a pair of $\XCal_T\times\YCal_T$-valued random variables with  $Law(X_T,Y_T)\in\mathcal{P}(\XCal_T\times\YCal_T)$. A loss functional $\mathcal{L}_T$ over $A_T$ is said to be {\em proper} with respect to $(X,Y)$ if there exist a corresponding function $L_T:\YCal_T\times\YCal_T\to\mathbb{R}$ bounded from below such that for any $f\in A_T$,
    \[\LL_T(f)=\E[L_T(Y,f(X))]=\E[\E[L_T(Y,f(X))|X]];\]
    moreover, the function $\tilde L_T:\YCal_T\to\mathbb{R}$ given by
    \[\tilde L_T(y)=\E[L_T(Y,Y')|Y'=y],\quad\forall y\in\YCal_T,\]
    is continuous. 
\end{defn}
Examples of proper loss functions include mean squared error and KL-divergence and more generally the Bregman divergence, assuming that the first and second moments of $Y$ conditioned on $Y'=y$ is continuous with respect to $y$. 
 
Without loss of generality,  we shall in this section assume the input transport set $\T^X$ contains all functions from $\XCal_T$ to $\XCal_S$. We then specify the following assumptions for the well-definedness of \eqref{eq: doub-trans}.
\begin{asp}\label{asp: A}
Assume the following regularity conditions hold.
\begin{enumerate}
    \item $\LL_T$ is a proper loss functional with respect to $(X_T,Y_T)$;
    \item the image $f_S^*(\XCal_S)$ is compact in $(\YCal_S,\|\cdot\|_{\YCal_S})$;
    \item the set $\T^Y$ is such that the following set of functions
    \[\tilde\T^Y=\{\tilde T^Y:\XCal_T\to\YCal_T\,|\,\exists T^Y\in\T^Y\text{ s.t. }\tilde T^Y(x)=\inf_{y\in f_S^*(\XCal_S)}\tilde L_T(T^Y(x,y)),\ \ \forall x\in\XCal_T\}\]
    is compact in $(\{f|f:{\XCal_T}\to\YCal_T\},\|\cdot\|_{\infty})$, where for any $f:\XCal_T\to\YCal_T$, $\|f\|_{\infty}:=\sup_{x\in\XCal_T}\|f(x)\|_{\YCal_T}$.
\end{enumerate}
\end{asp}
The proper choice of loss functions for $\mathcal{L}_T$ is fairly general and  includes the mean squared error, the KL-divergence, and more generally the Bregman divergence;  
the compactness assumptions can be fairly flexible as long as  the target optimal model $f_T^*$ can be written as
$f_T^*(x)=T^Y(x,f_S^*(T^X(x))),\quad\forall x\in\XCal_T.$
This compactness condition can be implemented by choosing a particular family of activation functions or imposing boundaries restrictions to weights and biases when constructing machine learning models. 

Now we are ready to prove Theorem \ref{thm:existence} under Assumption \ref{asp: A}.
\begin{proof}[Proof of Theorem \ref{thm:existence}]
Since $\LL_T$ is proper, there exists a function $L_T:\YCal_T\times\YCal_T\to\mathbb{R}$ such that 
\[\inf_{(y,y')\in\YCal_T\times\YCal_T}L_T(y,y')>-\infty,\]
and
\[\LL_T(T^Y(\cdot,(f_S^*\circ T^X)(\cdot)))=\E[L_T(Y_T,T^Y(X_T,(f_S^*\circ T^X)(X_T)))],\quad \forall T^X\in\T^X,\,T^X\in\T^X.\]
Therefore, for the function $\tilde L_T(\cdot)=\E[L_T(Y,Y')|Y'=\cdot]$, there exists $m\in\R$ such that $\tilde L_T(y)\geq m$ for any $y\in\YCal_T$.

Now fix any $T^Y\in\T^Y$. The continuity of $\tilde L_T$ and the continuity of $T^Y(x,\cdot)$ for each $x\in\XCal_T$ guarantee the continuity of $\tilde L_T(T^y(x,\cdot))$. Together with the compactness of $f_S^*(\XCal_S)$, we have that for any $x\in\XCal_T$, 
\[M_x=\argmin_{y\in f_S^*(\XCal_S)}\tilde L_T(T^Y(x,y))\neq\emptyset.\]
Therefore, for any $T^Y$, one can construct $\tilde T^{X}\in\T^X$ such that $\tilde T^X(x)\in M^x_{T^Y}$ for any $x\in\XCal_T$ and 
\[\min_{T^X\in\T^X}\LL_T(T^Y(\cdot,(f_S^*\circ T^X)(\cdot)))=\E[\tilde L_T(\tilde T^Y(X_T))]=:\tilde\LL_T(\tilde T^Y).\]
The continuity of the new loss functional $\tilde\LL_T$ comes from the continuity of the function $\tilde L$, and the particular choice of the function space $(\{f|f:{\XCal_T}\to\YCal_T\},\|\cdot\|_{\infty})$, where $\{f|f:{\XCal_T}\to\YCal_T\}$ contains all functions from $\XCal_T$ to $\YCal_T$. Since $\tilde\T^Y$ is compact in $(\{f|f:{\XCal_T}\to\YCal_T\},\|\cdot\|_{\infty})$, the minimum over $\tilde\T^Y$ is attained at some $\tilde T^{Y,*}$. According to the definition of $\tilde\T^Y$, there exists $T^{Y,*}\in\T^Y$ such that $\tilde T^{Y,*}(\cdot)=\inf_{y\in f_S^*(\XCal_S}T^{Y,*}(\cdot,y)$. Let $T^{X,*}$ be the $\tilde T^X\in\T^X$ corresponding to $T^{Y,*}$. For any $T^X\in\T^X$ and $T^Y\in\T^Y$, we have
\[\begin{aligned}
    \LL_T(T^Y(\cdot,(f_S^*\circ T^X)(\cdot)))&\geq \LL_T(T^Y(\cdot,(f_S^*\circ \tilde T^X)(\cdot)))\\
    &=\tilde \LL_T(\tilde T^Y(\cdot))\geq \tilde\LL_T(\tilde T^{Y,*}(\cdot))\\
    &=\LL_T(T^{Y,*}(\cdot,(f_S^*\circ T^{X,*}))(\cdot))\geq \min_{T^X\in\mathbb{T}^X,T^Y\in\mathbb{T}^Y}\LL_T\left(T^Y(\cdot, (f_S^*\circ T^X)(\cdot))\right).
\end{aligned}\]
Therefore, the transfer learning problem \eqref{eq: doub-trans} is well-defined and it attains its minimum at $(T^{X,*},T^{Y,*})$ described above. 
\end{proof}
If one removes the compactness assumptions in Assumption (A), then a sufficiently rich family of output transport mappings is needed, 
%i.e., $\T^Y=\{f|f:\XCal_T\times\YCal_S\to\YCal_T\}$, 
such that the target optimal model $f_T^*$ can be written as
$f_T^*(x)=T^Y(x,f_S^*(T^X(x))),\quad\forall x\in\XCal_T.$
However, it is often difficult to verify if the set $\T^Y$ is sufficiently rich, due to the construction of neural networks as well as the choices of optimization algorithms.  The compactness conditions, on the other hand, can be implemented through choosing a particular family of activation functions or imposing boundaries restrictions to weights and biases when constructing machine learning models.
